# Supplementary material for: Wave Tracing: Generalizing The Path Integral To Wave Optics
Source: arXiv:2508.17386 ancillary file (2025-08-24)
Supplement: Supplementary file 1 [file supplemental.pdf]

# Wave Tracing: Generalizing The Path Integral To Wave Optics — Supplemental

SHLOMI STEINBERG, University of Waterloo, Canada  
MATT PHARR, NVIDIA, United States

## S1 Analysis of the Classical Path Integral

We supplement the discussion from the paper, Section 3, where we study what optical phenomena can be reproduced by the classical path integral. We provide formal proofs and derivations here.

### S1.1 Geometric Propagation of Electromagnetic Fields

We discuss the conditions under which an electromagnetic field can be written as a field where wavefronts' propagation is point-wise governed by the geometric-optical Eikonal equation.

Let the electric and magnetic fields of some monochromatic radiation be

$$\vec{E}(\vec{r}, t) = \vec{a}(\vec{r})e^{iku(\vec{r})}e^{-i\omega t} \quad \text{and} \quad \vec{H}(\vec{r}, t) = \vec{h}(\vec{r})e^{iku(\vec{r})}e^{-i\omega t}, \quad (1)$$

where  $k = \frac{2\pi}{\lambda}$  is the (vacuum) wavenumber and  $\omega = ck$  is the temporal angular frequency, with  $\lambda$  being the (vacuum) wavelength and  $c$  speed of light in vacuum,  $\vec{a}, \vec{h}$  are real vector-valued spatial functions and  $u$  describes the field propagation dynamics: surfaces where  $u(\vec{r}) = \text{const}$  are the wavefronts, with  $\nabla u$  being the normals to these wavefronts—understood as direction of propagation of the wavefront. These are general expressions, since the complex spatial phase was decoupled from the other terms.

Let the fields above propagate in a medium with spatially-varying permittivity  $\epsilon(\vec{r})$  and permeability  $\mu(\vec{r})$ , and away from charge and current. Using Maxwell's equations, we get:

$$0 = \nabla \cdot \vec{E} = \left( \nabla \cdot \vec{a} + ik\vec{a} \cdot \nabla u \right) e^{iku} e^{-i\omega t} \quad (2)$$

$$0 = \nabla \cdot \vec{H} = \left( \nabla \cdot \vec{h} + ik\vec{h} \cdot \nabla u \right) e^{iku} e^{-i\omega t} \quad (3)$$

$$-\mu \frac{\partial \vec{H}}{\partial t} = \nabla \times \vec{E} = \left( \nabla \times \vec{a} + ik\vec{a} \times \nabla u \right) e^{iku} e^{-i\omega t} \quad (4)$$

$$\epsilon \frac{\partial \vec{E}}{\partial t} = \nabla \times \vec{H} = \left( \nabla \times \vec{h} + ik\vec{h} \times \nabla u \right) e^{iku} e^{-i\omega t}. \quad (5)$$

Assume that the spatial derivatives of  $\vec{a}$  and  $\vec{h}$  vanish or are negligible compared with dot or cross products above. We discuss the validity domain of this assumption later. Then, dropping these terms and simplifying gives

$$\nabla u \cdot \vec{E} = 0, \quad \nabla u \cdot \vec{H} = 0, \quad (6)$$

$$\nabla u \times \vec{E} = \omega\mu\vec{H}, \quad \nabla u \times \vec{H} = -\omega\epsilon\vec{E}. \quad (7)$$

By substituting Eq. (7) into each other and simplifying, we get:

$$k^2 \eta^2 \vec{E} = -\nabla u \times (\nabla u \times \vec{E}) = \vec{E} |\nabla u|^2, \quad (8)$$

with a similar relation for  $\vec{H}$ , where  $\eta = c\sqrt{\epsilon\mu}$  is the *refractive index*. We used the triple cross product identity, and the fact that  $\nabla u \cdot \vec{E} = 0$

(from Eq. (6)). The vacuum wavenumber  $k$  makes the wavelength dependence explicit.

Eq. (8) is the *Eikonal equation*  $|\frac{1}{k}\nabla u|^2 = \eta^2$ , with  $\nabla u(\vec{r})$  being the direction of propagation of the wavefront at  $\vec{r}$ , implying propagation is governed point-wise by geometric optics laws. The only assumption we made was neglecting the divergences and curls of  $\vec{a}, \vec{h}$  in Eqs. (2) to (5), which formally can be written as:

$$\nabla \cdot \vec{a} = 0 \quad \text{and} \quad |\nabla \times \vec{a}| \ll k|\vec{a} \times \nabla u|, \quad (9)$$

and similarly for  $\vec{h}$ . For which electromagnetic fields does this apply? A combination of far-field time-harmonic fields—arising far away from emitters or scattering matter—and sufficiently high spatial frequency fields (short wavelength).

Other work in optical literature has also analyzed electromagnetic fields, in order to derive some correspondence to a classical theory. For example, in the context of radiative transfer theory [Mishchenko et al. 2018].

*As a plane wave in the far field.* Finally, observe from the conclusions above that  $\{\vec{a}, \vec{h}, \nabla u\}$  form an orthogonal triad, and that the spatial variations in the peak amplitude and field directions  $\vec{a}, \vec{h}$  are small with respect to the spatial frequency  $k$ . Therefore, locally (and around a point to a second-order expansion) the field behaves as a plane wave.

*S1.1.1 As a wave ensemble.* Subsection S1.1 treated the fields as deterministic. Generalizing to a stochastic wave ensemble is straightforward: the above analysis applies for each realization of the wave ensemble, with identical conclusions.

In the paper, we also require that sensors time average over sufficiently long periods, thereby cross-spectral samples exhibit no interference at the sensor (i.e., paths of different wavelength are summed up linearly). For that to hold, time averaging must correspond to averaging over the wave ensemble statistics. This implies that the wave ensemble is *ergodic*, and ensemble averaging indeed becomes time averaging. Often, an assumption of stationarity (at least in the wide sense) is imposed as well, indicating that the temporal statistics of the field remain constant; though, as long as the time averaging period of the sensor is always greater than the ensemble's length of temporal coherence, stationarity is not strictly necessary.

Anyhow, the assumptions of ergodicity (and stationarity) are often well justified for optical fields [Wolf 1982]. Indeed, it is the assumptions on the electromagnetic field (on each realization of the wave ensemble) made in this Section that are far more constraining.

### S1.2 Scattering by a Surface

For simplicity, we perform our analysis with scalar fields. Let an incident local plane wave of wavenumber  $k$ ,  $\psi(\vec{r}) = e^{ik\vec{i}\cdot\vec{r}}$ , interact with a scattering surface. The incident and scattering directions are

Authors' Contact Information: Shlomi Steinberg, p@shlomisteinberg.com, University of Waterloo, Waterloo, Canada; Matt Pharr, matt@pharr.org, NVIDIA, San Francisco, United States.

$\vec{i}, \vec{o}$ , respectively. The (unknown) interaction region over the surface is  $A$ , and  $\alpha(\vec{r})$  be a modulation function that quantifies the scattered amplitude at a surface position. We formalize the interaction via the Fraunhofer diffraction integral:

$$I_o \propto \frac{1}{|A|} \left| \int_A \psi(\vec{r}) \alpha(\vec{r}) e^{ik\vec{o} \cdot \vec{r}} d\vec{r} \right|^2, \quad (10)$$

up to irrelevant constants.

To make further progress, we understand the surface scattering as a stationary, at least in the wide sense, random process with autocorrelation  $R_\alpha(\vec{r}_1 - \vec{r}_2) = \langle \alpha(\vec{r}_1) \alpha^*(\vec{r}_2) \rangle_m$ , where  $\langle \cdot \rangle_m$  indicates averaging over the material properties. Then, the scattered intensity in expectation is

$$\begin{aligned} \langle I \rangle_m &\propto \frac{1}{|A|} \left\langle \int_A \int_A \psi(\vec{r}_1) \psi^*(\vec{r}_2) \alpha(\vec{r}_1) \alpha^*(\vec{r}_2) e^{ik\vec{o} \cdot (\vec{r}_1 - \vec{r}_2)} d\vec{r}_1 d\vec{r}_2 \right\rangle_m \\ &= \frac{1}{|A|} \int_A \int_A R_\alpha(\vec{r}_1 - \vec{r}_2) e^{ik(\vec{i} + \vec{o}) \cdot (\vec{r}_1 - \vec{r}_2)} d\vec{r}_1 d\vec{r}_2. \end{aligned} \quad (11)$$

When the integration region  $A$  is sufficiently large to fully capture the statistics of the wide-sense stationary  $\alpha$ , by the Wiener–Khinchin theorem the Fourier transform above (after a change of variables to integrate over the lag  $\vec{r}_1 - \vec{r}_2$ ) yields the spectral power density  $S_\alpha$  of the random process:

$$\langle I \rangle_m \propto S_\alpha(k\vec{i} + k\vec{o}) \quad (12)$$

(up to irrelevant constants). We conclude that when  $\alpha$  is a (wide-sense stationary) random process, the expected scattered intensity is proportional to the spectral power density, assuming that  $A$  is much larger than the correlation length of the process.

In a like fashion, similar results are drawn for vectorized fields and volumetric interactions. Also, a more sophisticated diffraction method may be used, but the same conclusion applies: exact knowledge of  $A$  is not needed, as long as it is large enough such that autocorrelation  $R_\alpha$  dictates the integration range in Eq. (11).

**S1.2.1 Incoherence on Scattering.** We extend the analysis above to consider the scattered intensity when light illuminates the surface from two directions. We will show that the scattered intensity is an incoherent superposition of the incident waves.

Assume that light is observed at a single point far from the scattering surface. Let  $\vec{i}_1, \vec{i}_2, \vec{o}_1, \vec{o}_2$  be the incident and scattered directions, respectively, for the waves. Let  $\alpha$  and  $\alpha'$  be the random processes quantifying the scattering by the surface of the first and second plane waves, respectively. The regions of interaction are  $A_1, A_2$  for each of the incident waves, and we assume for simplicity that  $|A_1| = |A_2|$ . Then, the observed intensity is:

$$\begin{aligned} \langle I \rangle_m &\propto \frac{1}{|A_1|} \left\langle \left| \int_{A_1} e^{ik\vec{i}_1 \cdot \vec{r}} \alpha_1(\vec{r}) e^{ik\vec{o}_1 \cdot \vec{r}} d\vec{r} + \int_{A_2} e^{ik\vec{i}_2 \cdot \vec{r}} \alpha_2(\vec{r}) e^{ik\vec{o}_2 \cdot \vec{r}} d\vec{r} \right|^2 \right\rangle_m \\ &= \langle I_1 \rangle_m + \langle I_2 \rangle_m + 2 \operatorname{Re} \Im_{12} \end{aligned} \quad (13)$$

(up to irrelevant constants), where we expand the magnitude squared into a product, as before, and  $\langle I_{1,2} \rangle_m$  are the scattered intensities for each wave. The cross term between the integrals is:

$$\Im_{12} = \frac{1}{|A_2|} \int_{A_1} \int_{A_2} R_{12}(\vec{r}_1 - \vec{r}_2) e^{ik\vec{i}_1 \cdot (\vec{r}_1 + \vec{o}_1)} e^{-ik\vec{i}_2 \cdot (\vec{r}_2 + \vec{o}_2)} d\vec{r}_1 d\vec{r}_2$$

$$\begin{aligned} &= \frac{1}{|A_2|} \int_{A_2} e^{ik\vec{u} \cdot (\vec{i}_1 + \vec{o}_1 - \vec{i}_2 - \vec{o}_2)} d\vec{u} \int_{A_1 - A_2} R_{12}(\vec{v}) e^{ik\vec{v} \cdot (\vec{i}_1 + \vec{o}_1)} d\vec{v} \\ &= S_{12}(k\vec{i}_1 + k\vec{o}_1) \frac{1}{|A_2|} \int_{A_2} e^{ik\vec{u} \cdot (\vec{i}_1 + \vec{o}_1 - \vec{i}_2 - \vec{o}_2)} d\vec{u}, \end{aligned} \quad (14)$$

where  $R_{12} = \langle \alpha_1 \alpha_2^* \rangle_m$  is the cross-correlation between the random processes  $\alpha_1, \alpha_2$ , and  $S_{12}$  is the cross-spectral power density of the processes. We make the variable changes  $\vec{r}_1 - \vec{r}_2 \rightarrow \vec{v}$  and  $\vec{r}_2 \rightarrow \vec{u}$ , with  $A_1 - A_2 = \{\vec{r}_1 - \vec{r}_2 \mid \vec{r}_1 \in A_1, \vec{r}_2 \in A_2\}$ , and assume, as before, that the integral over  $\vec{v}$  fully captures the statistics of the scattering random process (note that the area  $|A_1 - A_2|$  is greater or equal to the areas of  $A_1, A_2$ ).

Consider the integral over  $A_2$  in the last equation above, and for simplicity we will analyze it in 2-dimensional space. Denote  $\vec{\zeta} = \vec{i}_1 + \vec{o}_1 - \vec{i}_2 - \vec{o}_2$  and let  $\zeta_x$  be its projection upon the (1-dimensional) surface. Then,  $\frac{1}{|A_2|} \int_{A_2} \exp(ik\vec{x}\zeta_x) dx = \operatorname{sinc}(\frac{k\zeta_x A_2}{2})$ . Over a two-dimensional surface this becomes a sinc squared. By our far-field assumption, we assume high-frequency radiation,  $k \gg 1$ , and large integration region,  $A_2 \gg 1$ , therefore the squared sinc term decays to 0 extremely rapidly as  $\vec{\zeta} \neq 0$ . Clearly, in our configuration,  $\vec{\zeta} = 0$  iff  $\vec{i}_1 = \vec{i}_2$  and  $\vec{o}_1 = \vec{o}_2$ .

We conclude that the cross term  $\Im_{12}$  vanishes, unless  $\vec{i}_1 = \vec{i}_2$  and  $\vec{o}_1 = \vec{o}_2$ , i.e. both waves arrive and scatter into the same direction, which also implies that  $\alpha_1 = \alpha_2$  and therefore  $S_{12}$  is the spectral power density of the random process. Therefore, the addition in Eq. (13) is always incoherent, with no interference. The same conclusion would not hold if we had explicit scattering features, which would limit the integration in Eq. (14) to a small extent. We did not make any new assumptions in this Section: we rely on the same far-field assumption, where the local plane wave resemblance of the high-frequency electromagnetic field is maintained over sufficiently large extents, and the wide-sense stationarity of the scattering random processes.

### S1.3 Proof of Conditions

We prove that subject to the following conditions (as presented in the paper), classical path tracing can reproduce the effects discussed in the paper in Section 3:

- (1) Light that is an ergodic, wide-sense stationary wave ensemble, of sufficiently large spatial frequencies.
- (2) Sensors that time average over periods long with respect to light's temporal coherence.
- (3) The far-field assumption is made several times: the points of a sampled path  $\vec{x}$  are assumed to be far from each other.
- (4) Scattering that is formulated in expectation by statistically wide-sense stationary materials only.

The wavefronts of an electromagnetic field that fulfills the postulates in Subsection S1.1 can be propagated, point-wise, using geometrical-optics rays. Let  $\vec{x} = \vec{x}_0 \vec{x}_1 \dots \vec{x}_n$  be a path constructed by such ray queries. At each interaction point  $\vec{x}_j$ , light is scattered by a wide-sense stationary random process, as in Eq. (12). Because the initial phase of the wavefront plays no role in the scattering, the scattered intensity, at path vertex  $\vec{x}_j$  is

$$I_o = I_i S_j(k\vec{i}_j + k\vec{o}_j), \quad (15)$$

where  $I_i$  is the incident intensity, and  $\vec{i}_j, \vec{o}_j$  are incident and scattering directions, and  $S_j$  is the material's power spectral density (PSD), as before. As the PSDs must be real and non-negative, the path contribution  $f(\vec{x})$  is also a real, non-negative value.

Let  $\vec{y}$  be another path. We want to show that the total contribution of  $\vec{x}, \vec{y}$  is incoherent, and no observable wave interference between the paths arises. If the paths are of different wavelength, then incoherence is mandated by the time-averaging of our sensors. Otherwise, assuming that lights interacts with the scene at least once, the paths always admit subpaths of the form  $\vec{x}_{j-1}\vec{x}_j\vec{z}$  and  $\vec{y}_{l-1}\vec{y}_l\vec{z}$ , with  $\vec{z}$  a common vertex. Then decoherence arises on scattering at  $\vec{x}_j$  and  $\vec{y}_l$ , which can be arbitrary vertices on the same or distinct materials, as discussed in Subsection S1.2.1. We conclude that the contribution of both paths is simply the incoherent sum  $f(\vec{x}) + f(\vec{y})$ , as required.

Above and in Subsection S1.2.1, we assume that a sufficiently diffuse interaction is taking place. In the case, where the emitter is imaged directly or through several perfectly (or almost perfectly) specular interactions, conditions on the emitter could be established for decoherence; we ignore this case as exceptional.

#### S1.4 What May Not Be Reproduced

Optical effects that cannot be reproduced accurately include all materials which may not be described as a stationary (at least in the wide sense) stochastic process. That is, any materials that include explicit scattering features. Such materials would require integration over infinite extents (in a sense, this can be understood as forcing stationary statistics from explicit data) which would imply an (impossible) infinite far-field assumption.

Some optical effects only arise over explicit realizations of the material's stochastic process (stationary or otherwise), but not in expectation. For example, optical speckle may materialize on scattering by a rough surface. While the surface might very well be described by a stationary process, when the scattering is formulated as the expected value, as in Eq. (11), no optical speckle would be reproduced. This is because we are averaging over the ensemble of all surface realization, but speckle requires integrating over a specific surface realization. The same applies to all other effects that do not arise in expectation.

Interference between materials (stationary or otherwise) cannot be reproduced (unless the interference process itself can be written as one material with an underlying stationary process; for example, thin film iridescence). This includes interference between geometric edges and geometric diffractions.

Finally, interference between spectral samples, and other temporal interference effects cannot be reproduced.

#### S2 Non-Negativity of the Bilinear Path Integral

Here we briefly prove the no-negativity of our bilinear generalization of the path integral (Subsection 4.1 in the paper).

Recall the properties of the mutual contribution function  $F$ :

$$F(\vec{x}, \vec{x}) \geq 0 \quad (16)$$

$$|F(\vec{x}, \vec{y})|^2 \leq F(\vec{x}, \vec{x})F(\vec{y}, \vec{y}), \quad (17)$$

i.e., it is non-negative over a single path and fulfills the Cauchy–Schwarz inequality. From the above we may deduce

$$\begin{aligned} & F(\vec{x}, \vec{x}) + F(\vec{y}, \vec{y}) + F(\vec{x}, \vec{y}) + F(\vec{y}, \vec{x}) \\ & \geq F(\vec{x}, \vec{x}) + F(\vec{y}, \vec{y}) - 2\sqrt{F(\vec{x}, \vec{x})F(\vec{y}, \vec{y})} \\ & = \left[ \sqrt{F(\vec{x}, \vec{x})} - \sqrt{F(\vec{y}, \vec{y})} \right]^2 \geq 0. \end{aligned} \quad (18)$$

Then, apply the bilinear path integral (Eq. (2) in the paper):

$$\begin{aligned} I &= \int_{\Omega \times \Omega} F(\vec{x}, \vec{y}) d\mu(\vec{x}) d\mu(\vec{y}) \\ &= \frac{1}{2} \int_{\Omega} d\mu(\vec{x}) \int_{\Omega \setminus \{\vec{x}\}} [F(\vec{x}, \vec{x}) + F(\vec{y}, \vec{y}) + F(\vec{x}, \vec{y}) + F(\vec{y}, \vec{x})] d\mu(\vec{y}) \\ &\geq 0, \end{aligned} \quad (19)$$

which concludes the proof.

Note that the property of non-negativity (Eq. (16)) follows from the Cauchy–Schwarz inequality (Eq. (17)); in the paper we make it explicit for clarity. Also note that the property of symmetry is not required for the proof above, however non-symmetric mutual contribution functions do not make physical sense.

#### S3 Background: Physical Light Transport

Physical light transport (PLT) works with Gaussian wave packets—termed *generalized rays* in Steinberg et al. [2024a]. Their name refers to the fact that generalized rays form the most compact, physically-realizable wave packets possible, and they generalize many of the useful properties of the classical ray of geometric optics to a wave optics. Nevertheless, generalized rays are not *rays*, per se—they are not infinitesimal rays with zero cross section—but a wave packet with a positive cross section. We refer to them as *Gaussian beams* to make the distinction from rays explicit. Formally, the phase-space distribution—the *Wigner distribution function* (WDF)—of such a Gaussian beam is

$$\begin{aligned} \phi_{\Sigma, \rho}(\vec{x}, \vec{k}; \vec{x}_0, \vec{k}_0) &\triangleq \frac{1}{\pi^3} \exp \left[ -(\vec{x} - \vec{x}_0)^\top \Sigma^{-1} (\vec{x} - \vec{x}_0) \right] \\ &\quad \times \exp \left[ -(\vec{k} - \vec{k}_0)^\top (\rho^2 \Sigma^{-1} + \Sigma) (\vec{k} - \vec{k}_0) \right] \\ &\quad \times \exp \left[ 2(\vec{x} - \vec{x}_0)^\top \rho \Sigma^{-1} (\vec{k} - \vec{k}_0) \right], \end{aligned} \quad (20)$$

and its corresponding (spatial) wave function takes the form:

$$\begin{aligned} \psi_{\Sigma, \rho}(\vec{x}; \vec{x}_0, \vec{k}_0) &\triangleq \frac{|\text{Re}(\Sigma + i\rho \mathbf{I})^{-1}|}{\pi^3} e^{i\vec{k}_0 \cdot (\vec{x} - \vec{x}_0)} \\ &\quad \times e^{-\frac{1}{2}(\vec{x} - \vec{x}_0)^\top (\Sigma + i\rho \mathbf{I})^{-1} (\vec{x} - \vec{x}_0)}, \end{aligned} \quad (21)$$

where  $\mathbf{I}$  is the identity matrix. In the definitions above,  $\vec{x}_0$  and  $\vec{k}_0$  are the *mean spatial position* and *mean wavevector*, respectively. Often, we will omit these means from the argument lists, for brevity.

The above parameterization of Gaussian beams is chosen in a way that is most compatible with how we use them in light transport simulations:  $\Sigma$  is the initial spatial variance (symmetric positive-definite) matrix of the wave packet, and  $\rho \geq 0$  is a correlation factor that depends on propagation distance (initially  $\rho = 0$  and it grows linearly with the distance travelled by the wave packet).  $\Sigma$  does not change on free-space propagation, but it may mutate upon light-matter interactions. We will discuss these aspects later.

By design, a decomposition into Gaussian beams admit properties that are very useful for light transport simulations: Gaussian beams are *weakly-local*, superpose *linearly* in terms of intensity observed by a sensor, and form a *complete* basis.

In general, transformation of the WDF—on propagation or interaction with matter—is described via an *interaction kernel*  $K$  and a corresponding *interaction operator*  $\mathcal{T}$ :

$$\mathcal{T}\{\mathcal{W}\}(\vec{x}, \vec{k}) \triangleq \int d^3\vec{x}' d^3\vec{k}' K(\vec{x}, \vec{x}', \vec{k}, \vec{k}') \mathcal{W}(\vec{x}', \vec{k}'), \quad (22)$$

where  $\mathcal{W}$  is an arbitrary WDF.  $K(\vec{x}, \vec{x}', \vec{k}, \vec{k}')$  can be understood as the impulse response arising at target point  $\vec{x}$  with wavevector  $\vec{k}$  under excitation from  $\vec{x}'$  with wavevector  $\vec{k}'$ .

For more information on WDFs in the optical context, see Bastiaans [1979]; Zhang and Levoy [2009].

## S4 Wave Tracing

### S4.1 Gaussian Beams as Elliptical Cones

The weak-locality of Gaussian beams means that we may define a geometric *envelope*—outside of which the wave packet is zero or negligible—and use that envelope for propagation and intersection tests with geometric meshes in our light transport simulations. We show that an *elliptical cone* serves as a tight geometric envelope.

Consider a Gaussian beam, with its phase space distribution quantified by Eq. (20). Via trivial analysis the first-order moments are

$$\int d^3\vec{x} d^3\vec{k} \vec{x} G_{\Sigma, \rho}(\vec{x}, \vec{k}) = \vec{x}_0 \quad (23)$$

$$\int d^3\vec{x} d^3\vec{k} \vec{k} G_{\Sigma, \rho}(\vec{x}, \vec{k}) = \vec{k}_0, \quad (24)$$

i.e. the mean spatial position and wavevector, as expected. The second-order moments (spatial and wavevector variances) are

$$\text{Var}_{\vec{x}} \triangleq \int d^3\vec{x} d^3\vec{k} \vec{x} \vec{x}^\top G_{\Sigma, \rho}(\vec{x}, \vec{k}) - \vec{x}_0 \vec{x}_0^\top = \frac{\rho^2}{2} \Sigma^{-1} + \frac{1}{2} \Sigma \quad (25)$$

$$\text{Var}_{\vec{k}} \triangleq \int d^3\vec{x} d^3\vec{k} \vec{k} \vec{k}^\top G_{\Sigma, \rho}(\vec{x}, \vec{k}) - \vec{k}_0 \vec{k}_0^\top = \frac{1}{2} \Sigma^{-1}. \quad (26)$$

We may recall the famous *uncertainty relation* [Mandel and Wolf 1995, Chapter 21]:  $|\text{Var}_{\vec{x}} \text{Var}_{\vec{k}}|^{1/2} \geq \frac{1}{2^3}$ , and note that (i) the variances above indeed fulfil this relation (because  $\rho \geq 0$ ); and, (ii) when  $\rho = 0$  (i.e., initially at sourcing, before the Gaussian beam has propagated) the equality in the uncertainty relation is fulfilled, meaning that Gaussian beams are *as spatially compact as physically permissible*.

In similar manner, we note that the correlation between the spatial position and wavevector dimensions is

$$\text{Corr}_{\vec{x}\vec{k}} \triangleq \int d^3\vec{x} d^3\vec{k} \vec{x} \vec{k}^\top G_{\Sigma, \rho}(\vec{x}, \vec{k}) - \vec{x}_0 \vec{k}_0^\top = \frac{\rho}{2} \Sigma^{-1}, \quad (27)$$

i.e., zero initially, and grows linearly with  $\rho$ .

We will now analyze how the Gaussian beam  $\phi$  transforms on free-space propagation. The free-space propagation kernel is

$$K(\vec{x}, \vec{x}', \vec{k}, \vec{k}') \triangleq \delta(\vec{k} - \vec{k}') \delta\left(\vec{x} - \frac{d}{|\vec{k}'|} \vec{k}' - \vec{x}'\right) \quad (28)$$

(see Testorf et al. [2010]), where  $\vec{d}$  is the distance of propagation. Start with  $\rho = 0$  (i.e. before propagation), then, via Eq. (22):

$$\phi'_{\Sigma, 0}(\vec{x}, \vec{k}) = \int K \times \phi_{\Sigma, 0} = \phi_{\Sigma, 0}\left(\vec{x} - \frac{d}{k} \vec{k}, \vec{k}\right). \quad (29)$$

Primed variables are used in order to denote quantities after the free-space propagation interaction. It is easy to verify that after propagation the spatial mean is translated by distance  $d$ , in direction of  $\vec{k}_0$  and the wavevector mean remains unchanged, as expected. The variances and covariances after propagation are

$$\text{Var}'_{\vec{x}} = \frac{1}{2} \frac{d^2}{k_0^2} \Sigma^{-1} + \frac{1}{2} \Sigma, \quad (30)$$

$$\text{Var}'_{\vec{k}} = \frac{1}{2} \Sigma^{-1}, \quad (31)$$

$$\text{Corr}'_{\vec{x}\vec{k}} = \frac{1}{2} \frac{d}{k_0} \Sigma^{-1}. \quad (32)$$

The above are identical to variances and covariances of the Gaussian beam  $\phi$  (Eqs. (25) to (27)) with  $\rho \equiv \frac{d}{k_0}$ . We conclude that on free-space propagation of distance  $d$  the correlation factor  $\rho$  increases by  $\frac{d}{k_0}$ .

As also observed by Man'ko and Wolf [2008], we note in passing that propagation induces correlation between position and momentum (wavevector), with  $\text{Corr}_{\vec{x}\vec{k}}$  increasing linearly with travel distance  $d$ . This correlation is responsible to the increase in the spatial extent occupied by the beam (as evident from Eq. (25)). It also means that we may not “break” a Gaussian beam into smaller beams after propagation, as these would not fulfil the uncertainty relation scaled by the induced correlation factor.

*Geometric interpretation.* Note that the spatial variance, Eq. (25), can be written as  $\text{Var}_{\vec{x}} = \frac{1}{2} \Sigma + \rho^2 \text{Var}_{\vec{k}}$ . The wavevector variance hence acts as the (potentially anisotropic) solid angle into which the wave packet propagates. Therefore, the three-dimensional ellipse  $\{\vec{x} \mid [(\vec{x} - \vec{x}_0)^\top \text{Var}_{\vec{x}} (\vec{x} - \vec{x}_0)]^{1/2} < 3\}$  formalises the spatial extent around the mean  $\vec{x}_0$  where the Gaussian beam wave packet is non-negligible (i.e., within 3 standard deviations in any direction). On propagation, with  $\rho = d/k_0$ , that ellipse traces an elliptical cone and forms a tight envelope (every point on the elliptical cone's shell is always within 3 standard deviations from the beam's mean) around the Gaussian beam.

As discussed in the paper, after interactions we do the following: in order to maintain the correlation factor between position and wavevector and produce correct beams and envelopes, we source a beam from the interaction region, projected into the new direction of propagation. This fixes the spatial variance for the new beam, and the wavevector variance—the solid angle into which the beam propagates—remains identical to the incident beam.

### S4.2 Bi-Directional Light Transport

Light transport with Gaussian beams was formalized for backward-only transport [Steinberg et al. 2024a], i.e. where sensor distributions are transformed via time-reversed interactions, and then integrated over emission distributions (formally, a functional inner product):

$$I = (2\pi)^3 \left\langle \mathcal{W}_e, \left( \mathcal{T}_{b, N_b}^\top \circ \dots \circ \mathcal{T}_{b, 1}^\top \right) \left\{ \mathcal{W}_d \right\} \right\rangle, \quad (33)$$

where  $I$  is the observed intensity by the sensor,  $\mathcal{W}_e, \mathcal{W}_d$  are the sensor and emitter distributions, i.e. their WDFs, respectively ( $d$  stands for

“detector”, and  $e$  stands for “emitter”), and  $\mathcal{T}_{b,j}^{-t}$  is a sequence of  $N_b \geq 0$  *time-reversed interaction operators* ( $b$  stands for “backward”): in practice, these are sequences of free-space propagations followed by light-matter interactions. See Steinberg et al. [2024a, Section 4] for more information on these interactions.

In similar manner, we may apply forward (non time-reversed) interactions to the emitter distribution, giving rise to *bi-directional* light transport formulation:

$$I = (2\pi)^3 \left\langle \left( \mathcal{T}_{f,N_f} \circ \dots \circ \mathcal{T}_{f,1} \right) \left\{ \mathcal{W}_e \right\}, \left( \mathcal{T}_{b,N_b}^{-t} \circ \dots \circ \mathcal{T}_{b,1}^{-t} \right) \left\{ \mathcal{W}_d \right\} \right\rangle. \quad (34)$$

We decompose the sensor and emitter distributions into linear sums of Gaussian beams:

$$\mathcal{W}_d = \sum_{m=1}^{M_d} I_d^{(m)} \phi_{\Sigma_d^{(m)},0} \quad \text{and} \quad (35)$$

$$\mathcal{W}_e = \sum_{l=1}^{M_e} I_e^{(l)} \phi_{\Sigma_e^{(l)},0}, \quad (36)$$

with  $I_{d,e}$  being the power contained in each beam. Gaussian beams sourced from an emitter remain weakly-local and linear.

For any interaction operator  $\mathcal{T}$  and beam  $\phi$ , the transformed distribution  $\mathcal{T}\{\phi\}$  can always be written as a sum of one or more Gaussian beams [Steinberg et al. 2024a]. Therefore, the problem of integrating Eq. (34) reduces to integrating two Gaussian beams with identical wavevectors (i.e., the distributions are propagated towards each other, and time-reversal flips the wavevector), propagated to the same mean position:

$$\begin{aligned} \langle \phi_{\Sigma_1,\rho_1}, \phi_{\Sigma_2,\rho_2} \rangle &= \int d^3\vec{x} d^3\vec{k} \phi_{\Sigma_1,\rho_1}(\vec{x},\vec{k}) \phi_{\Sigma_2,\rho_2}(\vec{x},\vec{k}) \\ &= 2^3 \frac{|\Sigma_1|^{1/2} |\Sigma_2|^{1/2}}{|\det[\Sigma_1 + \Sigma_2 + i(\rho_1 - \rho_2)I]|}, \end{aligned} \quad (37)$$

where in the denominator we take the complex magnitude of the determinant.

The variances  $\Sigma_d^{(m)}$  of Gaussian beams that are sourced from a sensor are chosen such that the spatial extent coincides with the size of the sensor (or pixel), or a part of it. How do we choose the variances  $\Sigma_e^{(l)}$  of the Gaussian beams sourced from the emitter? Ideally, we would like to maximise the contribution of connected Gaussian beams, i.e. maximize Eq. (37). In general, that requires intimate knowledge of the entire transport that both Gaussian beams (forward and backward) take before integration. Bereft of such information, we note that one way to maximise Eq. (37) is when  $\rho_1 = \rho_2$  and  $\Sigma_1 = \Sigma_2$ . That is, if we initially set  $\Sigma_1 = \Sigma_2$ , and if we assume that the travel distance of the forward and backward Gaussian beams is roughly similar, viz.  $\rho_1 \approx \rho_2$ . If we assume that light-matter interactions only apply orthogonal transformations to the variances  $\Sigma_{1,2}$  (which is often, but not always, the case), then Eq. (37) takes its maximal value of 1.

**Summary.** Bi-directional transport with Gaussian beams involves:

- (1) Sampling a Gaussian beam from an emitter distribution, and propagating and transforming it *forward* in the scene.

- (2) Sampling a Gaussian beam from a sensor distribution, and propagating and transforming it *backward*, via time-reversed temporal dynamics time-reversed interaction operators.
- (3) Connecting the backward and forward Gaussian beams by propagating both towards each other (opposite wavevectors) and to the same spatial position, and integrating their contribution via Eq. (37).

Note that the above is similar to classical bi-directional light transport: Sensor and emitter light subpaths are constructed, and then connected to form a complete emitter-to-sensor light path. The primary differences compared with the classical formalism are:

- In the classical case the throughput of a connection between the sensor and emitter subpaths is either 0 (shadowed) or 1; in our case, a connection requires propagating the Gaussian beams towards each other, and (if no shadowing occurs) the throughput is the integral over the Gaussian beams’ phase space footprint and may take any value in  $[0, 1]$ .
- Due to the above, multiple importance sampling (MIS) of the subpath connection strategies becomes more complicated, and is left for future work.
- Typically, in the classical context the generation of the emitter subpath does not depend on the sensor to which we attempt to connect, however in our case the spatial variance  $\Sigma_e^{(l)}$  of the emitted Gaussian beam is chosen w.r.t. the sensor.

### S4.3 Interaction with Matter

We will now consider the interaction of a Gaussian beam with matter. Let a Gaussian beam impinge upon matter with different scattering potential functions  $h_1, \dots, h_N$  that dictate the scattering from different spatial regions (i.e., different materials that fall within the Gaussian beam’s envelope). The aggregated interaction kernel, for the entire region under the Gaussian beam spatial extent, can be written as [Testorf et al. 2010]

$$\begin{aligned} K(\vec{x}, \vec{x}', \vec{k}, \vec{k}') &= \int d^3\vec{y} d^3\vec{y}' \exp(-i\vec{k} \cdot \vec{y} + i\vec{k}' \cdot \vec{y}') \\ &\times \sum_j h_j(\vec{x} + \tfrac{1}{2}\vec{y}, \vec{x}' + \tfrac{1}{2}\vec{y}') \sum_l h_l^*(\vec{x} - \tfrac{1}{2}\vec{y}, \vec{x}' - \tfrac{1}{2}\vec{y}'), \end{aligned} \quad (38)$$

where  $h_j$  are the optical response functions of the matter. The above motivates us to define *cross-interaction kernels*:

$$\begin{aligned} K_{jl}(\vec{x}, \vec{x}', \vec{k}, \vec{k}') &\triangleq \int d^3\vec{y} d^3\vec{y}' \exp(-i\vec{k} \cdot \vec{y} + i\vec{k}' \cdot \vec{y}') \\ &\times h_j(\vec{x} + \tfrac{1}{2}\vec{y}, \vec{x}' + \tfrac{1}{2}\vec{y}') h_l^*(\vec{x} - \tfrac{1}{2}\vec{y}, \vec{x}' - \tfrac{1}{2}\vec{y}'). \end{aligned} \quad (39)$$

We denote the shorthand  $K_j \equiv K_{jj}$ . While the interaction kernels  $K$  and  $K_j$  are real functions, the cross-interaction kernels  $K_{jl}$  (with  $j \neq l$ ) typically take complex values.

The aggregated interaction kernel is then

$$K \triangleq \sum_j K_j + \sum_{j \neq l} K_{jl} = \sum_j K_j + 2 \operatorname{Re} \sum_{l > j} K_{jl}, \quad (40)$$

where the second equality follows from the fact that  $K_{jl} = K_{lj}^*$ . Two kinds of terms enter Eq. (40): (i) *Direct kernels*  $K_j$ : these quantify the wave-optical interaction with a single material (e.g., a single triangle)—in a sense, the wave-optical analogue of the classical BSDF. Examples of interaction operators are provided by [Steinberg et al.

2024a, Supplemental]. (ii) *Cross terms*  $K_{jl}$ : these account for the interference between each pair of materials.

Let  $\mathcal{T}$  be the aggregated interaction operator that corresponds to the kernel  $K$ . Let the incident Gaussian beam be  $\phi_{\Sigma', \rho'}$ . The power contained in a scattered Gaussian beam is then the inner product

$$I\{\phi_{\Sigma, \rho}\} = \langle \phi_{\Sigma', \rho'}, \mathcal{T}\{\phi_{\Sigma, \rho}\} \rangle = \int d^3\vec{x} d^3\vec{k} d^3\vec{x}' d^3\vec{k}' \\ \times \phi_{\Sigma, \rho}(\vec{x}, \vec{k}) K(\vec{x}, \vec{x}', \vec{k}, \vec{k}') \phi_{\Sigma', \rho'}(\vec{x}', \vec{k}'). \quad (41)$$

Further analytic progress requires making some assumptions with regards to the kernels  $K, K_{jl}$ .

*Quasi-homogeneous matter.* Often, we are interested in describing the matter statistically: for example, a rough surface, participating medium or a diffraction grating; and computing the scattering response in expectation. In such cases, we understand the scattering potentials  $h_j$  as stochastic processes. A useful class of statistical matter is *quasi-homogeneous scatterers* [Korotkova 2017, Chapter 8.2] (introduced as locally-stationary matter by Steinberg and Yan [2021]), where the cross-correlation between a pair of scattering potentials  $h_j, h_l$  can be written as:

$$\langle h_j(\vec{x}_1, \vec{x}_1') h_l^*(\vec{x}_2, \vec{x}_2') \rangle \\ = I_{jl} \left( \frac{\vec{x}_1 + \vec{x}_2}{2}, \frac{\vec{x}_1' + \vec{x}_2'}{2} \right) \mu_{jl}(\vec{x}_2 - \vec{x}_1, \vec{x}_2' - \vec{x}_1'), \quad (42)$$

where  $\langle \cdot \rangle$  denotes ensemble averaging (not to be confused with the inner product).  $\vec{x}', \vec{x}$  can be understood as source and destination positions, respectively,  $I_{jl}$  is the scattering mutual intensity, and  $\mu_{jl}$  is the *degree of spatial cross-correlation*. When  $j = l$  the cross-correlation of the scattering process above becomes the auto-correlation. Dependence on wavenumber  $k$  is implied.

The ensemble-averaged cross-interaction kernels in Eq. (39) become

$$\langle K_{jl}(\vec{x}, \vec{x}', \vec{k}, \vec{k}') \rangle = I_{jl}(\vec{x}, \vec{x}') \tilde{\mu}_{jl}(\vec{k}, \vec{k}'), \quad (43)$$

where  $\tilde{\mu}$  is defined as the conjugated double Fourier transform of the degree of cross-correlation:

$$\tilde{\mu}_{jl}(\vec{k}, \vec{k}') \triangleq \int d^3\vec{y} d^3\vec{y}' e^{-i\vec{k} \cdot \vec{y} + i\vec{k}' \cdot \vec{y}'} \mu_{jl}(\vec{y}, \vec{y}'). \quad (44)$$

For more information on locally-stationary matter, see Steinberg and Yan [2021, Section 5].

#### S4.4 Fraunhofer Materials

We define a special case of quasi-homogeneous matter as *Fraunhofer kernels*. Such kernels arise when two conditions are met: (i) the mutual intensities  $I_{jl}$  do not depend on the destination position  $\vec{x}$ , viz.

$$I_{jl}(\vec{x}, \vec{x}') \equiv I_{jl}(\vec{x}'), \quad (45)$$

(ii) and, in Eq. (43), we may replace the  $K(\vec{x}, \vec{x}', \vec{k}, \vec{k}')$  term with  $K(\vec{x}, \vec{x}', \vec{k}_0, \vec{k}'_0)$ , where  $\vec{k}_0, \vec{k}'_0$  are the mean wavevectors before and after interaction. These assumptions can be understood as the Fraunhofer approximation for quasi-homogeneous matter, and is a form of a far field assumption. Interactions such as scattering by rough surfaces, diffraction gratings, and many optical elements can be represented by Fraunhofer kernels.

Then, for such kernels,

$$\langle I\{\phi_{\Sigma, \rho}\} \rangle = \sum_{jl} \tilde{\mu}_{jl}(\vec{k}_0, \vec{k}'_0) \int d^3\vec{x} d^3\vec{k} \phi_{\Sigma, \rho}(\vec{x}, \vec{k}) \\ \times \int d^3\vec{x}' d^3\vec{k}' I_{jl}(\vec{x}') \phi_{\Sigma', \rho'}(\vec{x}', \vec{k}'). \quad (46)$$

Note that  $\int \phi = 1$ , by definition, hence the integral over  $\vec{x}, \vec{k}$  is unity:

$$\langle I\{\phi_{\Sigma, \rho}\} \rangle = \sum_{jl} \tilde{\mu}_{jl}(\vec{k}_0, \vec{k}'_0) \int d^3\vec{x}' d^3\vec{k}' I_{jl}(\vec{x}') \phi_{\Sigma', \rho'}(\vec{x}', \vec{k}') \\ = \sum_{jl} \tilde{\mu}_{jl}(\vec{k}_0, \vec{k}'_0) \langle \phi_{\Sigma', \rho'}, I_{jl} \rangle, \quad (47)$$

i.e., the inner product of the incident Gaussian beam with the scattering mutual intensities  $I_{jl}$ , times the degrees-of-spatial cross-correlations  $\tilde{\mu}_{jl}$ .

*Relation to the classical BSDF.* Let

$$I_{jl}(\vec{x}') = \begin{cases} 1 & \text{if } j = l \text{ and } \vec{x}' \in S_j \\ 0 & \text{otherwise} \end{cases} \quad (48)$$

$$\tilde{\mu}_{jj}(\vec{k}, \vec{k}') = f_j(\vec{k}, \vec{k}'), \quad (49)$$

where  $S_j \subset \mathcal{R}^3$  is the scattering matter (e.g., a triangle), and  $f_j$  is the classical BSDF (with the cosine foreshortening factored in).  $I_{jl} \equiv 0$  (for  $j \neq l$ ) implies that no cross-interaction interference arises (a consequence of classicality). Then, Eq. (50) becomes

$$\langle I\{\phi_{\Sigma, \rho}\} \rangle = \sum_j f_j(\vec{k}_0, \vec{k}'_0) \langle \phi_{\Sigma', \rho'}, I_{jl} \rangle, \quad (50)$$

where the inner product is now the integration of the incident Gaussian beam over the triangle, multiplied by the classical BSDF  $f$ .

#### S4.5 Importance sampling strategy

We detail the general importance sampling strategy for the multi-material wave-optical interactions, that was presented in the paper. We assume that an importance sampling strategy for each direct term  $K_j$  (i.e., for a single material) is given to us. Then, note that

$$\forall j, l \ K_{jl} = 0 \rightarrow K_j = 0 \quad (51)$$

$$\text{and } \forall \vec{x}, \vec{x}', \vec{k}, \vec{k}', \ K \leq N \sum_j K_j, \quad (52)$$

where  $N$  is the count of interactions  $K_j$ , and Eq. (52) is derived via application of the Cauchy-Schwarz inequality to  $(\sum h_j)(\sum h_l)^*$  in Eq. (40). Hence, the incoherent (interference-neglecting) sum of direct terms  $\sum_j K_j$  serves as a proposal distributions for the aggregated kernel  $K$ .

Let  $\mathcal{T}_{jl}$  be the interaction operator that corresponds to the cross-interaction kernel  $K_{jl}$ . Our importance sampling strategy is:

- (1) Draw a wavevector  $\vec{k}$  by importance sampling the incoherent sum of direct terms  $\sum_j \mathcal{T}_{jj}$ .
- (2) Let  $I_1, I_2$  be the powers in  $\sum_j \mathcal{T}_{jj}\{\phi\}$  and the aggregated term  $\mathcal{T}\{\phi\}$ , respectively, for sampled  $\vec{k}$ .
- (3) Rejection sample [Casella et al. 2004]:
  - (a) Draw uniform  $u \in [0, 1]$ .
  - (b) If  $u < I_2/(NI_1)$  accept  $\vec{k}$ , otherwise return to step 1.

That is, we importance sample from the direct terms (similar to sampling from classical BSDFs in computer graphics), and rejection sample in order to account for the cross-material interference. The number of iterations of step 3 above is, on average,  $N$ : the count of different interactions that fall within the Gaussian beam's footprint. Correctness is ensured by Eqs. (51) and (52).

The strategy above is presented in its utmost generality, and is designed to work with arbitrary operators  $\mathcal{T}$  and  $\mathcal{T}_{jl}$ .

## S5 The Weakly-Local Path Integral

Our weakly-local generalization of the path integral takes the form

$$I = \int_{\Omega} g(\bar{\mathbf{R}}) d\mu(\bar{\mathbf{R}}) . \quad (53)$$

As in the paper,  $\bar{\mathbf{R}} = \mathbf{R}_0 \mathbf{R}_1 \dots \mathbf{R}_k$  is a *generalized path* defined as sequence of bounded regions  $\mathbf{R}_j \subset \mathbb{R}^3$ . The set  $\Omega_1$  of all bounded subsets  $\mathbf{R}_j \subset \mathbb{R}^3$  is trivially (Lebesgue) measurable, therefore the Cartesian product

$$\Omega_k = \underbrace{\Omega_1 \times \dots \times \Omega_1}_{k \text{ times}} \quad (54)$$

is trivially measurable, and the set of all possible generalized paths  $\bar{\mathbf{R}}$  of all finite lengths  $k$ , viz.

$$\Omega = \bigcup_k \Omega_k \quad (55)$$

is a measurable set, and the measure  $\mu$  on  $\Omega$  is the appropriate product measure.  $g$  is the *path contribution function*, written in operator form:

$$g(\bar{\mathbf{R}}) = W T_{\mathbf{R}_{n-2} \rightarrow \mathbf{R}_{n-1} \rightarrow \mathbf{R}_n} T_{\mathbf{R}_{n-3} \rightarrow \mathbf{R}_{n-2} \rightarrow \mathbf{R}_{n-1}} \dots T_{\mathbf{R}_0 \rightarrow \mathbf{R}_1 \rightarrow \mathbf{R}_2} L_{\mathbf{R}_0 \rightarrow \mathbf{R}_1}(\mathbf{R}_0) , \quad (56)$$

where  $T$  are generic transport operators,  $L$  is a sourcing function and  $W$  is a generic measurement operator that must yield a non-negative scalar.

**S5.0.1 Local Path Sampling.** Monte Carlo integration of Eq. (53) is identical to the classical case:

$$I \approx \sum_{n=1}^N \frac{g(\bar{\mathbf{R}}_n)}{p_n} . \quad (57)$$

A strength of our path integral formulation is that the intermediate distributions that are sourced via  $L$ , transformed via  $T$  and then measured via  $W$  are not directly needed to construct a path: the sequence of regions  $\mathbf{R}_j$  defines the path. Only once a path  $\bar{\mathbf{R}}_n = \mathbf{R}_0 \mathbf{R}_1 \dots \mathbf{R}_k$  is constructed, the light transport over that path needs to be evaluated via  $g(\bar{\mathbf{R}}_n)$ .

Without explicitly defining the co-domain of  $L$ , we may define an *intensity operator*:

$$I_0 = \mathcal{I} \{ L_{\mathbf{R}_0 \rightarrow \mathbf{R}_1}(\mathbf{R}_0) \} , \quad (58)$$

which quantifies the non-negative power contained in the sourced distribution  $L_{\mathbf{R}_0 \rightarrow \mathbf{R}_1}(\mathbf{R}_0)$ , given  $\mathbf{R}_0, \mathbf{R}_1$ , regardless of the analytic nature of  $L_{\mathbf{R}_0 \rightarrow \mathbf{R}_1}(\mathbf{R}_0)$  and the used optical formalism. Local path sampling then proceeds classically: Sample the initial pair of regions  $\mathbf{R}_0$  and  $\mathbf{R}_1$ ; in practice, in our formalism this is done by sampling a *minimum-uncertainty* ( $\rho = 0$  in Eq. (20)) Gaussian beam from the source (fixing  $\mathbf{R}_0$ ), sampling an initial wavevector  $\vec{\mathbf{k}}$  from the

sensor's sensitivity function, and then wave tracing (as in the paper) in order to construct the next region  $\mathbf{R}_1$ .

After sampling the initial two regions, we need to sample  $\mathbf{R}_2$ . This is done by considering the intensity of the scattered distribution:

$$I_1 = \mathcal{I} \{ T_{\mathbf{R}_0 \rightarrow \mathbf{R}_1 \rightarrow \mathbf{R}_2} L_{\mathbf{R}_0 \rightarrow \mathbf{R}_1}(\mathbf{R}_0) \} . \quad (59)$$

For Fraunhofer materials (Subsection S4.4),  $I_1$  only depends on direction from  $\mathbf{R}_1$  to the (unknown) next region  $\mathbf{R}_2$ . Local path sampling then samples a new direction, and the region  $\mathbf{R}_2$  is constructed via wave tracing, as before. For example, if the material at  $\mathbf{R}_1$  is just a perfect mirror, then  $I_1$  is a Dirac as function of direction; if the material is a moderately-rough surface, then the angular distribution of power is proportional to a surface scattering theory (we use SPM surfaces)—how the surface transforms and mutates the light distribution is not relevant, only the total power in the scattered distribution. When multiple materials fall within an interaction region, our general importance sampling strategy, Subsection S4.5, is used. The process repeats recursively in order to sample a complete path  $\bar{\mathbf{R}}$ .

The above summarizes conceptually the sampling approach taken in Subsection S4.3: only the powers carried by the Gaussian beams, defined in Eq. (41), are considered for importance sampling and path construction. The rest of the properties of the Gaussian beams  $\phi$  are deduced geometrically via wave tracing. For non-Fraunhofer materials, the process is more involved, the powers  $I_j$  may now be functions of additional parameters, often the distance to next region. This happens with UTD-based diffraction methods, and importance sampling strategies for non-Fraunhofer materials are left for future work.

**S5.0.2 Non-Negativity of Measurement.** The non-negativity of the measurement function  $g$  depends on the light transport formalism. In our case, we work in the space-frequency (Wigner) space, therefore the measurement operator  $W$  is the inner product in Wigner space, as in the paper:

$$W\phi_k \equiv \langle W_s , \phi_k \rangle , \quad (60)$$

where  $W_s$  is the space-frequency sensitivity distribution of the sensor. The non-negativity of this measurement operator is an immediate consequence of Moyal's formula [Torre 2005].

For other formalisms, a different measurement is defined. For example, if the distributions  $\phi$  are wavefunctions (electric fields), then the measurement becomes

$$W\phi_k \equiv |\langle \psi_s , \phi_k \rangle|^2 , \quad (61)$$

where  $\psi_s$  is the sensor's response function (its Wigner distribution is  $W_s$ ), and non negativity is explicit.

## S6 Implementation Details

**Traversal.** We use an 8-wide SAH-based BVH for traversal [Emre et al. 2025]. The SAH cost ratio is skewed compared with ray tracing since the (AVX2 vectorized) 8-wide traversal is significantly faster than the expensive (exact and watertight) elliptical cone–triangle intersection tests. Thus, we use a large SAH cost ratio which tends to create deeper trees. The BVH also supports hybrid workloads—cone and ray tracing—which is important for ballistic propagation.

Ray tracing is fully vectorized (both traversal and intersection tests) as well.

Some cone tracing-specific BVH optimizations are done. One example is full-subtree traversal: if an elliptical cone fully contains a node, full intersection tests are not needed (we know the triangles are contained in the cone); instead the cone distances to all the triangles in the entire subtree are computed in a vectorized manner, and the triangles that fall within the intersection frustum are added to the list of intersected primitives. This gives a major speed-up in cases where cones fall upon fine geometric details.

**Spectral rendering.** Our renderer targets a wide range of applications across the EM spectrum. Each emitter and sensor define their spectral emission or sensitivity distributions. A variety of spectral distributions are supported: discrete, Dirac, uniform, piecewise linear, or Gaussian. Some more specialized analytic spectra, like blackbody emission, or ITU [ITU 2023] provided refractive indices are defined. Distributions can also be loaded from databases: e.g., XYZ sensitivity spectra for optical rendering, different emitter profiles, or index-of-refraction curves for different materials.

For each emitter–sensor pair, the product of their emission and sensitivity spectra is numerically integrated and is used for spectral importance sampling (and MIS). Each path only carries a single spectral sample; we do not use fixed bins, as that suffers from spectral aliasing, nor do we carry several spectral samples over a path, as the interactions that are hardest to spectrally integrate (dispersion and diffractions) are often dispersive anyway.

Some data can also be loaded from an image (texture); this is mostly relevant for optical applications. The image data is upsampled from RGB to spectral.

**Materials.** We support a limited set of materials. Surfaces use the small perturbation method (SPM) theory, are wavelength dependent, and provide simple support for slight-to-moderately rough surfaces. The surface profile is defined via its power spectral density, and can be a Dirac (perfectly specular), Gaussian or fractal (also known as the K-Correlation model) distribution. Of course, due to their wavelength dependence, surfaces that scatter in a rough manner at some spectral range are very smooth in other spectral ranges. Being statistically-stationary materials, we assume that no interference between such surfaces arises, simplifying the implementation. These surfaces also model dielectric interfaces, with transmission.

More targeted materials, like surface models for RF simulations that also model backscattering, are left for future work.

**Diffractions and interactions.** Every sample is propagated via its elliptical cone, as discussed in the paper, and the elliptical conic envelope fully defines the properties of the underlying Gaussian beam. Our renderer is polarimetric, and each sample’s power is quantified via its Stokes parameters vector. Interactions are naturally formulated via the Mueller-Stokes calculus.

As discussed in the paper, we support two modes of diffractions: Fraunhofer edge-based diffractions [Steinberg et al. 2024b] for optical applications, and UTD edge-based diffractions for longer wavelength simulations. When an elliptical conic envelope intersects geometry, we classify and keep track of the edges (according to the chosen diffraction method). For UTD, we limit wedge angles to  $160^\circ$ .

We importance sample a point on the beam’s cross section (with respect to the cross-sectional Gaussian distribution of intensity); if that point falls upon a surface, we importance that surface for the scattering direction; if free-space was sampled, then we importance sample the free-space diffraction operator (i.e., the entire cross-edge interference, using our importance sampling strategy in Subsection S4.5). We transform the beam, as in the paper, and wave trace to the next interaction region. If diffracting edges were detected in the previous region, we also evaluate the free-space diffraction operator (also when surface interactions were sampled).

**Polarization and emission.** The emitters used in this paper are simple isotropic emitters that are attached to a shape (area emitters) or simple point emitters. More sophisticated emitters, for example antenna arrays and non-isotropic antenna radiation patterns, are also left for future work.

## References

- M. J. Bastiaans. 1979. Wigner distribution function and its application to first-order optics. *J. Opt. Soc. Am.* 69, 12 (Dec 1979), 1710–1716. doi:10.1364/JOSA.69.001710
- George Casella, Christian P. Robert, and Martin T. Wells. 2004. *Generalized Accept-Reject sampling schemes*. Institute of Mathematical Statistics, 342–347. doi:10.1214/lnms/1196285403
- Umut Emre, Aryan Kanak, and Shlomi Steinberg. 2025. High-Performance Elliptical Cone Tracing. *Computer Graphics Forum* 44, 7 (Oct 2025). doi:10.1111/cgf.70230
- ITU. 2023. Recommendation ITU-R P.2040-3. [https://www.itu.int/dms\\_pubrec/itu-r/rec/p/R-REC-P.2040-3-202308-1!!PDF-E.pdf](https://www.itu.int/dms_pubrec/itu-r/rec/p/R-REC-P.2040-3-202308-1!!PDF-E.pdf)
- Olga Korotkova. 2017. *Random Light Beams*. CRC Press, Boca Raton.
- Leonard Mandel and Emil Wolf. 1995. *Optical coherence and quantum optics*. Cambridge University Press, Cambridge.
- Vladimir I Man’ko and Kurt Bernardo Wolf. 2008. The influence of spherical aberration on Gaussian beam propagation. In *Lie Methods in Optics*. Springer Berlin Heidelberg, Berlin, Heidelberg, 207–225.
- Michael I Mishchenko, Larry D Travis, and Andrew A Lacis. 2018. *Multiple scattering of light by particles*. Cambridge University Press, Cambridge, England.
- Shlomi Steinberg, Ravi Ramamoorthi, Benedikt Bitterli, Eugene d’Eon, Ling-Qi Yan, and Matt Pharr. 2024a. A Generalized Ray Formulation For Wave-Optical Light Transport. *ACM Trans. Graph.* 43, 6, Article 241 (Nov. 2024), 15 pages. doi:10.1145/3687902
- Shlomi Steinberg, Ravi Ramamoorthi, Benedikt Bitterli, Arshiya Mollazainali, Eugene D’Eon, and Matt Pharr. 2024b. A Free-Space Diffraction BSDF. *ACM Trans. Graph.* 43, 4, Article 113 (jul 2024), 15 pages. doi:10.1145/3658166
- Shlomi Steinberg and Ling-Qi Yan. 2021. Physical Light-Matter Interaction in Hermite-Gauss Space. *ACM Trans. Graph.* 40, 6, Article 283 (dec 2021), 17 pages. doi:10.1145/3478513.3480530
- Markus Testorf, Bryan Hennelly, and Jorge Ojeda-Castañeda. 2010. *Phase-space optics: fundamentals and applications*. McGraw-Hill Education.
- Amalia Torre. 2005. *Linear ray and wave optics in phase space: bridging ray and wave optics via the Wigner phase-space picture*. Elsevier.
- Emil Wolf. 1982. New theory of partial coherence in the space–frequency domain. Part I: spectra and cross spectra of steady-state sources. *J. Opt. Soc. Am.* 72, 3 (Mar 1982), 343–351. doi:10.1364/JOSA.72.000343
- Zhengyun Zhang and Marc Levoy. 2009. Wigner distributions and how they relate to the light field. In *2009 IEEE International Conference on Computational Photography (ICCP)*. 1–10. doi:10.1109/ICCPHOT.2009.5559007
